# Supplementary material for: Real-time exciton dynamics with time-dependent density-functional theory
Source: arXiv:2102.01796 ancillary file (2021-02-02)
Supplement: Supplementary file 1 [file supplemental.pdf]

# Supplemental material for: Real-time exciton dynamics with time-dependent density-functional theory

Jiuyu Sun,<sup>1,2</sup> Cheng-Wei Lee,<sup>3</sup> Alina Kononov,<sup>4</sup> André Schleife,<sup>3,5,6</sup> and Carsten A. Ullrich<sup>1</sup>

<sup>1</sup>*Department of Physics and Astronomy, University of Missouri, Columbia, Missouri 65211, USA*

<sup>2</sup>*Max Planck Institute for the Structure and Dynamics of Matter, 22761 Hamburg, Germany*

<sup>3</sup>*Department of Materials Science and Engineering,*

*University of Illinois at Urbana-Champaign, Urbana, Illinois 61801, USA*

<sup>4</sup>*Department of Physics, University of Illinois at Urbana-Champaign, Urbana, Illinois 61801, USA*

<sup>5</sup>*Materials Research Laboratory, University of Illinois at Urbana-Champaign, Urbana, Illinois 61801, USA*

<sup>6</sup>*National Center for Supercomputing Applications,*

*University of Illinois at Urbana-Champaign, Urbana, Illinois 61801, USA*

(Dated: February 2, 2021)

## I. IMPLEMENTATION OF THE SCALED ALDA

In the main paper, we define three types of exchange-correlation (xc) kernels: adiabatic LDA ( $f_{xc}^{ALDA}$ ), long-range corrected (LRC) ( $f_{xc}^{LRC}$ ), and the combined kernel  $f_{xc}^{LRC+} = f_{xc}^{LRC} + \beta f_{xc}^{ALDA}$ . Within linear-response (LR)-TDDFT, the implementation of these xc kernels is straightforward in the Yambo code [1]. However, in real-time (RT)-TDDFT using Qb@ll, the implementation of the  $\beta$ -scaled ALDA needs to be done with care, to ensure that the LR and RT formalisms are consistent.

The default implementation of the ALDA in Qb@ll involves the full xc potential  $v_{xc}^{ALDA}[n](t)$ , but the  $\beta$ -scaling only affects the response part associated with  $\delta n(t)$ , see Eq. (5) in the main paper. Let us consider the fundamental relationship  $f_{xc}^{ALDA}(\mathbf{r}, \mathbf{r}') = \delta v_{xc}^{ALDA}[n](\mathbf{r}) / \delta n(\mathbf{r}')|_{n_{gs}(\mathbf{r})}$ . Multiplying  $\beta$  on both sides, we have

$$\beta f_{xc}^{ALDA}(\mathbf{r}, \mathbf{r}') = \frac{\beta \delta v_{xc}^{ALDA}[n](\mathbf{r})}{\delta n(\mathbf{r}')}\bigg|_{n_{gs}(\mathbf{r})}. \quad (1)$$

This suggests the algorithm for RT-TDDFT with the  $\beta$ -scaled ALDA xc potential,  $v_{xc,\beta}^{ALDA}$ , described in the following pseudocode, where  $\Psi(t)$  denotes the Kohn-Sham wave function:

---

### Algorithm 1 $\beta$ -scaled ALDA xc potential

---

**Require:** ground state  $v_{xc}^{LDA}$ ,  $\Psi(0) = \Psi_{gs}$

**for**  $istep = 1 \rightarrow nsteps$  **do**

generate  $n(t)$  from  $\Psi(t)$

update  $v_{xc}^{ALDA}[n](t)$  with  $n(t)$

$\beta \delta v_{xc}^{ALDA}(t) = \beta [v_{xc}^{ALDA}[n](t) - v_{xc}^{LDA}]$

$v_{xc,\beta}^{ALDA}(t) = v_{xc}^{LDA} + \beta \delta v_{xc}^{ALDA}(t)$

propagate  $\Psi(t) \rightarrow \Psi(t + \Delta t)$  with  $v_{xc,\beta}^{ALDA}(t)$

$t = t + \Delta t$

**end for**

---

Notice that the parameter  $\beta$  can be set to zero, in which case  $f_{xc}^{LRC+}$  reduces to the pure LRC kernel  $f_{xc}^{LRC} =$

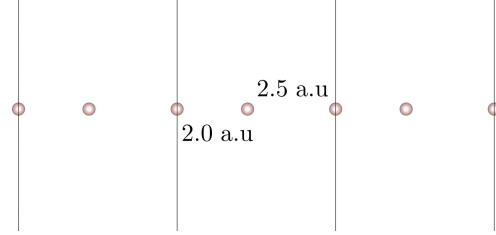

FIG. 1. Geometry of the molecular  $H_2$  chain, with lattice constant 4.5 a.u.

$-\alpha/k^2$ , and there are no dynamical corrections to the ground-state LDA xc potential; this is used for  $H_2$  chain in the main paper.

## II. COMPUTATIONAL DETAILS

### A. Real-time propagation with Qb@ll

Since it is more convenient to adopt an orthogonal unit cell in Qb@ll, we used a conventional cubic cell containing 8 Si atoms for Si and 4 Li and 4 F atoms for LiF, respectively, with the experimental lattice parameters. The  $H_2$  chain is set up to have a lattice constant of 4.5 a.u. (atomic units) along the periodic direction (see Fig. 1). For CsGeCl<sub>3</sub>, we adopted the cubic  $Pm\bar{3}m$  phase. The lattice constant is optimized (using the Quantum Espresso package [2], see below) to be 10.32 a.u., which is in agreement with results quoted in the literature [3].

With the geometries as defined above, we first calculate the Kohn-Sham ground state for all systems. A plane wave basis implementation (the default in Qb@ll) is employed, with cutoff energies of 20 Hartree for Si and 40 Hartree for the other three systems. Together with optimized norm-conserving Vanderbilt pseudopotentials [4, 5], we used the LDA functional for Si,  $H_2$  chain and LiF, and the PBE [6] functional for CsGeCl<sub>3</sub>. We used regular Monkhorst-Pack (M-P) meshes of  $64 \times 1 \times 1$ ,  $6 \times 6 \times 6$  and  $8 \times 8 \times 8$  for  $H_2$  chain, LiF and CsGeCl<sub>3</sub>, respectively. The  $\mathbf{k}$ -point meshes adopted for Si will be discussed in more detail in Section III below.

Starting from the ground state, the systems are excited in two different ways for the linear response and short-pulse response simulations, respectively. In the velocity gauge, see Eq. (4) in the main paper, a uniform external electric field  $\mathbf{E}'$  gives rise to a vector potential  $\mathbf{A}'(t)$ ,

$$\mathbf{A}'(t) = - \int^t \mathbf{E}'(t') dt', \quad (2)$$

and the single-particle Bloch functions acquire a phase factor when going from the length to the velocity gauge:

$$\varphi_j(\mathbf{r}, t) = e^{-i\mathbf{A}' \cdot \mathbf{r}} \tilde{\varphi}_j(\mathbf{r}, t). \quad (3)$$

For the former case, we adopted a delta-kick by a constant and uniform electric field  $\mathbf{E}'$  along the  $z$ -direction. This means that a constant  $\mathbf{A}'$  along the  $z$ -direction is turned on at the beginning of the propagation, i.e.  $\mathbf{A}'(t) = \text{const.}$  ( $t \geq 0$ ). To compare with LR calculations in the weakly perturbed regime, we chose small values of  $\mathbf{A}'$  of  $5 \times 10^{-3}$  a.u. for Si,  $\text{H}_2$  chain and  $\text{CsGeCl}_3$ , and  $5 \times 10^{-4}$  a.u. for LiF (which corresponds to electric field spikes of strength 2.6 and 0.26 V/nm, respectively).

A time step of 0.08 a.u. is employed for Si and LiF, and a time step of 0.05 a.u. for  $\text{H}_2$  chain and  $\text{CsGeCl}_3$ . A time propagation of at least 20 fs is performed for all the systems unless the simulation diverges. With the accumulated macroscopic total current density  $\mathbf{j}_0$  of every step, the dielectric response  $\varepsilon(\omega)$  is calculated via [7]

$$\varepsilon(\omega) = 1 + \frac{4\pi i \sigma(\omega)}{\omega}, \quad (4)$$

where the frequency-dependent conductivity is given by

$$\sigma(\omega) = -\frac{1}{A'} \int_{-T}^T e^{i\omega t} f(t) j_0(t) dt, \quad (5)$$

and  $f(t)$  is a suitably chosen window function. In order to compare with experimental or BSE results, the dielectric functions are corrected by rigid blue shifts of 0.6 eV, 3.05 eV, 5.4 eV and 1.6 eV for Si,  $\text{H}_2$  chain, LiF and  $\text{CsGeCl}_3$ , respectively.

For the nonlinear short-pulse response in Si, see Fig. 2 in the main paper, we used the same  $\mathbf{k}$ -grid as before. Instead of calculating the dielectric function and applying the scissors operator, we follow Ref. [8] and consider the dipole power spectrum (in the so-called acceleration form), following from the time-dependent induced current:

$$|P(\omega)|^2 = \left| FT \int_{\Omega} d\mathbf{r} \frac{\partial}{\partial t} \mathbf{j}(\mathbf{r}, t) \right|^2 \quad (6)$$

where  $FT$  stands for Fourier Transform. The dipole power spectrum has been widely used to study harmonic generation in atoms, molecules and, more recently, solids.

## B. Optical response with Yambo

We used the Yambo code [1] to perform LR-TDDFT and BSE calculations for optical excitations. The Kohn-Sham ground-state wave functions, used as input to Yambo, are calculated using the Quantum Espresso package [2]. Except for the  $\mathbf{k}$ -point mesh, we apply the same cubic cells and computational parameters, as well as the scissors operator, to keep consistent with Qb@ll. For the ground state and LR-TDDFT, we used  $\Gamma$ -centered meshes of  $64 \times 1 \times 1$ ,  $8 \times 8 \times 8$  and  $12 \times 12 \times 12$  for  $\text{H}_2$  chain, LiF and  $\text{CsGeCl}_3$ , respectively.

The RPA dielectric functions were calculated with at least 100 conduction bands and 123  $\mathbf{G}$ -vectors for Si. The corresponding numbers for the other materials are: 19 conduction bands and 1005  $\mathbf{G}$ -vectors for the  $\text{H}_2$  chain, 160 conduction bands and 200  $\mathbf{G}$ -vectors for LiF, and 160 conduction bands and 300  $\mathbf{G}$ -vectors for  $\text{CsGeCl}_3$ . For our LR-TDDFT calculations, these parameters are kept the same as for the RPA calculations for each material, except that we only use 1 conduction band for the  $\text{H}_2$  chain.

To build the BSE kernels, we used 4 valence and 4 conduction bands for Si. The corresponding numbers of valence and conduction bands for the other materials are: (1,1) for the  $\text{H}_2$  chain and (13,7) for  $\text{CsGeCl}_3$ . We used Haydock iteration to solve the BSE-type equations, instead of directly diagonalizing the huge BSE matrix.

Due to the absence of experimental data for the electronic band gap of  $\text{H}_2$  chain and cubic  $\text{CsGeCl}_3$ , we used the  $G_0W_0$  method to correct the quasiparticle energy. With the RPA dielectric function obtained above, we included 32 and 160 conduction bands for  $\text{H}_2$  chain and  $\text{CsGeCl}_3$ , respectively. The band gap correction for the  $\text{H}_2$  chain is 3.05 eV, which is applied as the magnitude of scissors shift in BSE. The BSE optical spectrum is in agreement with Ref. [9]. Thus we further applied this scissors shift for LR-TDDFT. The electronic band gap of cubic  $\text{CsGeCl}_3$  is corrected to be 2.96 eV, which is in agreement with previous work [3]. Thus a correction of 1.6 eV is then applied as a scissors shift for all optical spectra of  $\text{CsGeCl}_3$  with BSE and LR-TDDFT. Note here that the scissors shift is different from the rigid shift applied in RT-TDDFT [10, 11], though we adopted the same value for each material.

## III. MORE ON $\mathbf{k}$ -POINT SAMPLING

### A. $\mathbf{k}$ -point sampling for TDDFT

We carefully tested the  $\mathbf{k}$ -point sampling for calculating the dielectric function  $\text{Im}(\varepsilon)$  of Si (with an 8-atom unit cell). The calculations were performed with the Quantum Espresso package by using *pw.x* and *epsilon.x*, where the RPA level was constructed using Kohn-Sham ground-state wave functions. As shown in Fig. 2, we tested M-P  $\mathbf{k}$ -point meshes [12] from  $8^3$  up to  $42^3$ . It can

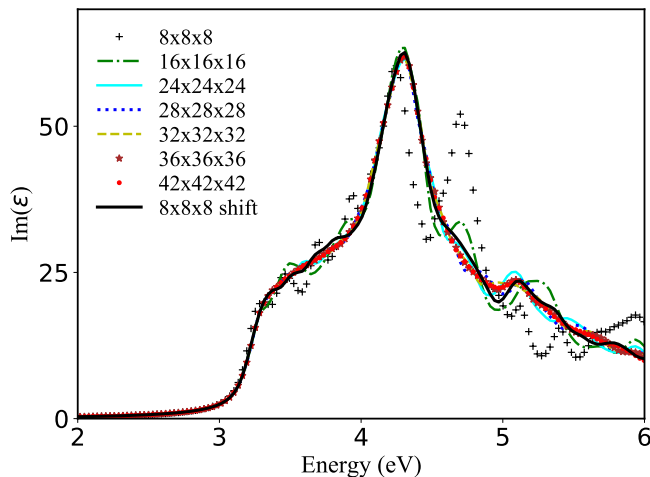

FIG. 2. RPA dielectric function  $\text{Im}(\epsilon)$  of Si calculated using different  $\mathbf{k}$ -point meshes with Quantum Espresso. A scissors shift of 0.6 eV is applied.

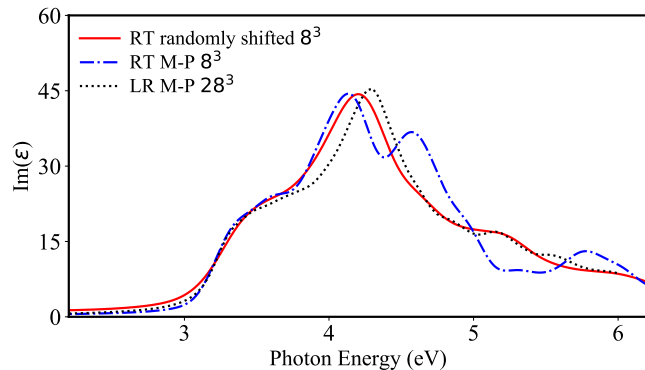

FIG. 3. Dielectric function  $\text{Im}(\epsilon)$  of Si calculated by RT ALDA with different  $8^3$   $\mathbf{k}$ -meshes, as well as LR ALDA with  $8^3$  M-P mesh. A scissors shift of 0.6 eV is applied.

be seen that  $\text{Im}(\epsilon)$  is not well converged until the  $\mathbf{k}$ -point mesh of  $28^3$  for the lower energy part below 4 eV. However, the higher energy part beyond 5.5 eV is still not converged even when the number of  $\mathbf{k}$ -points increases from  $36^3$  to  $42^3$ .

It has been reported in the literature that RT-TDDFT simulations can be sensitive to  $\mathbf{k}$ -point sampling [7]. In order to reduce the computational cost and keep the  $\mathbf{k}$ -point sampling still adequate, we applied an additional shift based on the  $8^3$  M-P mesh. The additional small shift by the reciprocal-space vector  $\mathbf{v} = (0.028526, 0.041304, 0.107901)$  is randomly generated. Then we applied the same random shift vector to every  $\mathbf{k}$ -point of the  $8^3$  M-P mesh. With the shifted  $8^3$  mesh, we obtained a curve of  $\text{Im}(\epsilon)$  (black solid line) similarly smooth as that by  $28^3$  (blue dotted line). Therefore, in the main paper we use this shifted  $8^3$  mesh for all the RT simulations of Si with Qb@ll.

However, randomly shifted meshes are unavailable in

the Yambo code, where we have to use a  $\Gamma$ -centered or M-P mesh. Based on the results above, we choose an M-P mesh of  $28^3$  for the LR-TDDFT calculations in Yambo. We compare  $\text{Im}(\epsilon)$  of Si calculated with different meshes in Fig. 3. For RT-TDDFT, the ALDA spectrum with the randomly shifted mesh is much improved compared to that calculated with a regular M-P mesh, especially for eliminating the artificial peak around 4.6 eV. In fact, RT-TDDFT with the randomly shifted mesh is similar to LR-TDDFT with the  $28^3$  mesh, which confirms our conclusions from the test above with Quantum Espresso.

The slight differences between the LR- and RT-TDDFT optical spectra of Si in Figs. 1 in the main paper can be mainly attributed to the use of different  $\mathbf{k}$ -meshes. Even though we obtained almost identical RPA results for the randomly shifted  $8^3$  mesh and the  $28^3$  M-P mesh, there is no guarantee that these two meshes work similarly for different TDDFT approaches. This is particularly pronounced for the  $\text{LRC}_+$  optical spectra of Si, where LR- and RT-TDDFT give overall similar results, but the  $E_1$  and  $E_2$  peaks are not quite aligned.

## B. $\mathbf{k}$ -point sampling for BSE

The M-P mesh of  $28^3$  gives well converged spectra, but we cannot use it for BSE calculations because of the huge cost for a unit cell containing 8 Si atoms. It is well known that a large number of  $\mathbf{k}$ -points, even much more than  $28^3$ , are required to obtain converged BSE spectra [13, 14]. We adopted the random integration method and inversion solver in Yambo [1, 15]. In this scheme, the BSE spectrum of Si is calculated with a double  $\mathbf{k}$ -grid, which includes a  $24 \times 24 \times 24$   $\Gamma$ -centered uniform  $\mathbf{k}$ -point mesh and 30000 random interpolated  $\mathbf{k}$ -points. In addition, we chose to use a primitive cell with 2 Si atoms for BSE calculations.

In Fig. 1 in the main paper, it is found that the BSE spectrum differs from the experiment by a lower  $E_1$  peak. At this stage, increasing the number of  $\mathbf{k}$ -points would be unlikely to improve the result. Other factors should be taken into account, for example dynamical effects in the screened electron-hole interaction, as discussed in detail in Ref. [16].

For  $\text{CsGeCl}_3$ , we also applied the double  $\mathbf{k}$ -grid technique, using a  $\Gamma$ -centered  $8^3$  uniform  $\mathbf{k}$ -mesh and 10000 random interpolated  $\mathbf{k}$ -points.

## IV. REAL-TIME CURRENT DENSITIES FOR Si, $\text{H}_2$ CHAIN AND LiF

In this section, we present the real-time total current densities ( $J_z$ ) of Si,  $\text{H}_2$  chain, LiF, and  $\text{CsGeCl}_3$ , which are not shown in the main paper. For Si, the results here are for linear response, excited by the delta-kicked electric field (the currents induced by femtosecond laser pulses are shown in Fig. 2a in the main paper).

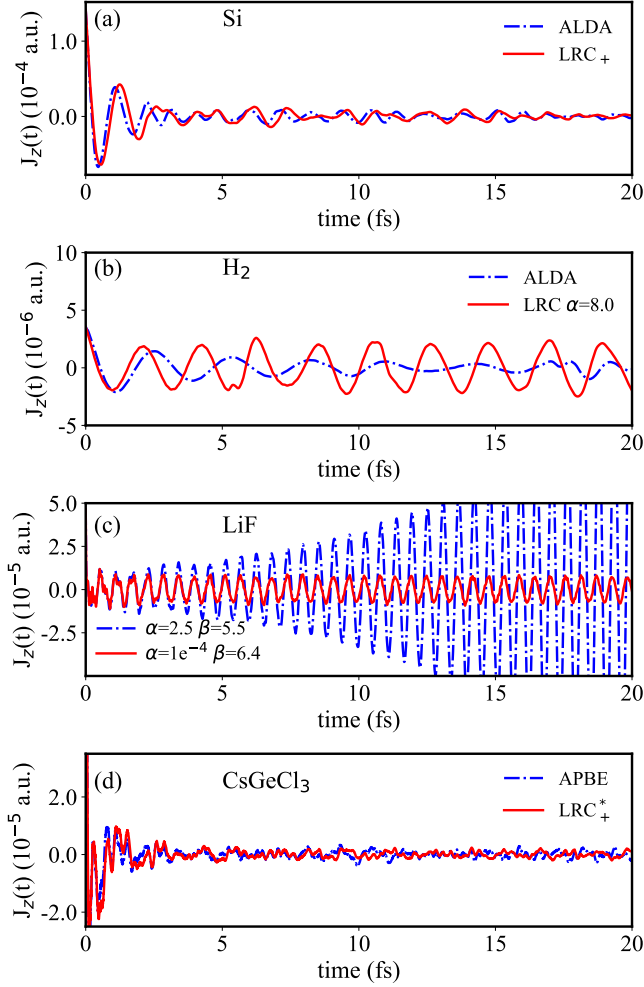

FIG. 4. Real-time current densities  $J_z$  calculated by RT-TDDFT for (a) Si (linear dielectric response), (b)  $H_2$  chain, (c) LiF and (d)  $CsGeCl_3$ .

In Fig. 4a, we compare the macroscopic  $J_z$  of Si generated by ALDA and  $LRC_+$  in the main paper. It can be seen that the oscillations of both current densities become much smaller after a time propagation of 20 fs. This is due to the fact that the exciton in Si is close to the conduction band continuum, which leads to a rather rapid dephasing of the induced current oscillations.

By contrast, in Fig. 4b for the  $H_2$  chain, the  $J_z$  generated by LRC with  $\alpha = 8.0$  exhibits a much stronger oscillation than  $J_z$  by ALDA, even no trend of decay. In the one-dimensional hydrogen chain, the exciton is strongly bound and has a large oscillator strength, which is reflected by the prominent oscillations in the current density.

In LiF, the frequencies of the current oscillations by  $LRC_+$  with  $(\alpha = 2.5, \beta = 5.5)$  and  $(\alpha = 10^{-4}, \beta = 6.4)$  are almost the same, which gives us the excitonic peaks so close to each other in energy (see Fig. 3c in the main paper). However, the oscillations of  $J_z$  for  $(\alpha = 2.5, \beta = 5.5)$  remain strong after 5 fs, which leads to a much higher peak in the optical spectrum. In addition, one can also observe an instability of the induced currents for  $(\alpha = 2.5, \beta = 5.5)$ .

For  $CsGeCl_3$ , the induced current densities are quite similar to those for Si discussed above, which is related to the fact that both systems have weakly bound excitons, close to or even partially embedded into the absorption continuum.

- 
- [1] D. Sangalli, A. Ferretti, H. Miranda, C. Attaccalite, I. Marri, E. Cannuccia, P. Melo, M. Marsili, F. Paleari, A. Marrazzo, G. Prandini, P. Bonfà, M. O. Atambo, F. Affinito, M. Palummo, A. Molina-Sánchez, C. Hogan, M. Grüning, D. Varsano, and A. Marini, Many-body perturbation theory calculations using the yambo code, *J. Phys.: Condens. Matter* **31**, 325902 (2019).
  - [2] P. Giannozzi, O. Andreussi, T. Brumme, O. Bunau, M. B. Nardelli, M. Calandra, R. Car, C. Cavazzoni, D. Ceresoli, M. Cococcioni, N. Colonna, I. Carnimeo, A. D. Corso, S. de Gironcoli, P. Delugas, R. A. D. Jr, A. Ferretti, A. Floris, G. Fratesi, G. Fugallo, R. Gebauer, U. Gerstmann, F. Giustino, T. Gorni, J. Jia, M. Kawamura, H.-Y. Ko, A. Kokalj, E. Küçükbenli, M. Lazzeri, M. Marsili, N. Marzari, F. Mauri, N. L. Nguyen, H.-V. Nguyen, A. O. de-la Roza, L. Paulatto, S. Poncé, D. Rocca, R. Sabatini, B. Santra, M. Schlipf, A. P. Seitsonen, A. Smogunov, I. Timrov, T. Thonhauser, P. Umari, N. Vast, X. Wu, and S. Baroni, Advanced capabilities for materials modelling with QUANTUM ESPRESSO, *J. Phys.: Condens. Matter* **29**, 465901 (2017).
  - [3] L.-y. Huang and W. R. L. Lambrecht, Electronic band structure trends of perovskite halides: Beyond Pb and Sn to Ge and Si, *Phys. Rev. B* **93**, 195211 (2016).
  - [4] D. R. Hamann, Optimized norm-conserving Vanderbilt pseudopotentials, *Phys. Rev. B* **88**, 085117 (2013), erratum: *ibid.* **95**, 239906 (2017).
  - [5] M. van Setten, M. Giantomassi, E. Bousquet, M. Verstraete, D. Hamann, X. Gonze, and G.-M. Rignanese, The pseudodojo: Training and grading a 85 element optimized norm-conserving pseudopotential table, *Comput. Phys. Commun.* **226**, 39 (2018).
  - [6] J. P. Perdew, K. Burke, and M. Ernzerhof, Generalized gradient approximation made simple, *Phys. Rev. Lett.* **77**, 3865 (1996), erratum: *ibid.* **78**, 1396 (1997).
  - [7] K. Yabana, T. Sugiyama, Y. Shinohara, T. Otake, and G. F. Bertsch, Time-dependent density functional theory for strong electromagnetic fields in crystalline solids,

- Phys. Rev. B **85**, 045134 (2012).
- [8] N. Tancogne-Dejean, O. D. Mücke, F. X. Kärtner, and A. Rubio, Impact of the electronic band structure in high-harmonic generation spectra of solids, Phys. Rev. Lett. **118**, 087403 (2017).
  - [9] D. Varsano, A. Marini, and A. Rubio, Optical saturation driven by exciton confinement in molecular chains: A time-dependent density-functional theory approach, Phys. Rev. Lett. **101**, 133002 (2008).
  - [10] Z. H. Levine and D. C. Allan, Linear optical response in silicon and germanium including self-energy effects, Phys. Rev. Lett. **63**, 1719 (1989).
  - [11] X. Gonze and C. Lee, Dynamical matrices, Born effective charges, dielectric permittivity tensors, and interatomic force constants from density-functional perturbation theory, Phys. Rev. B **55**, 10355 (1997).
  - [12] H. J. Monkhorst and J. D. Pack, Special points for Brillouin-zone integrations, Phys. Rev. B **13**, 5188 (1976).
  - [13] D. Rocca, Y. Ping, R. Gebauer, and G. Galli, Solution of the Bethe-Salpeter equation without empty electronic states: Application to the absorption spectra of bulk systems, Phys. Rev. B **85**, 045116 (2012).
  - [14] S. Albrecht, L. Reining, G. Onida, V. Olevano, and R. Del Sole, Albrecht et al. reply:, Phys. Rev. Lett. **83**, 3971 (1999).
  - [15] D. Kammerlander, S. Botti, M. A. L. Marques, A. Marini, and C. Attaccalite, Speeding up the solution of the Bethe-Salpeter equation by a double-grid method and Wannier interpolation, Phys. Rev. B **86**, 125203 (2012).
  - [16] A. Marini and R. Del Sole, Dynamical excitonic effects in metals and semiconductors, Phys. Rev. Lett. **91**, 176402 (2003).
